# Supplementary material for: Fractional Charges, Linear Conditions and Chemical Potentials for Excited States in $\Delta SCF$ Theory
Source: arXiv:2408.08443 ancillary file (2024-08-19)
Supplement: Supplementary file 1 [file SI_FractionalDeltaSCF2024.pdf]

# Supplemental Material: Fractional Charges, Linear Conditions and Chemical Potentials for Excited States in $\Delta SCF$ Theory


Weitao Yang

*Department of Chemistry and Department of Physics,*

*Duke University, Durham, North Carolina 27708*[*]

Yichen Fan

*Department of Chemistry, Duke University, Durham, North Carolina 27708*



[*] weitao.yang@duke.edu

## CONTENTS

I. 1-Particle Density Matrix of Entangled States 3
A. Half integers 3
B. All fractions 5
C. The contribution of the cross term to the total energy 5

II. Excited-State Chemical Concepts 7

III. Computational details and results for excitation energies of fractional charge systems 9
A. OH radical electron addition and removal 9
1. The molecular orbital diagram for the ground and excited states of OH radical/ion 9
2. Ground state electron addition and removal 11
3. Excited state to ground state electron addition and removal 14
4. Excited state to excited state electron addition and removal 17
5. Plot for the fractional charged system total energies with respect to the number of electrons. 18
B. Li atom electron addition and removal 19
1. Ground state electron addition and removal 20
2. Excited state to ground state electron addition and removal 22

IV. Comparison between EOM-CCSD and $\Delta SCF$ 23
A. OH radical/ion EOM-CCSD and $\Delta SCF$ comparision 23
B. Li atom/ion EOM-CCSD and $\Delta SCF$ comparision 25

References 25

## I. 1-PARTICLE DENSITY MATRIX OF ENTANGLED STATES

We provide details of the non-interacting density matrices for systems with subsystems separated by infinite distances and examine the contributions to total energy.

### A. Half integers

We will determine the density matrix for the $(2N+1)-$electron entangled wavefunctions $\Phi$ of the noninteracting reference system from the product states $\Psi_\alpha$ , $\Psi_\beta$ :

$$\Phi_\alpha = \hat{A}\left(\Phi_N^0\left(\mathbf{R}_1\right)\Phi_{N+1}^{n_s}\left(\mathbf{R}_2\right)\right), \tag{1}$$

$$\Phi_\beta = \hat{A}\left(\Phi_{N+1}^{n_s}\left(\mathbf{R}_1\right)\Phi_N^0\left(\mathbf{R}_2\right)\right), \tag{2}$$

$$\Phi = \left\{\Phi_\alpha + \Phi_\beta\right\}/\sqrt{2}, \tag{3}$$

where $n_s$ is the excitation number of the noninteracting reference system. The noninteracting wavefunctions $\Phi_\alpha$ and $\Phi_\beta$ have the same noninteracting eigenvalues, but are *not* degenerate wavefunctions of a single noninteracting reference Hamiltonian $H_s$. Instead, they are the eigenstates of two different noninteracting reference Hamiltonians: $\Phi_\alpha$ is an eigenstate of a $H_s$ with potential $w^0_{s,\mathbf{R}_1}(\mathbf{x}, N) + w^{n_s}_{s,\mathbf{R}_2}(\mathbf{x}, N+1)$, and $\Phi_\beta$ is an eigenstate of another $H_s$ with potential $w^{n_s}_{s,\mathbf{R}_1}(\mathbf{x}, N+1) + w^0_{s,\mathbf{R}_2}(\mathbf{x}, N)$, where we use the notation $w^{n_s}_{s,\mathbf{R}_2}(\mathbf{x}, N+1)$ to denote the local potential associated with the $n_s$th eigenstate $\Phi_{N+1}^{n_s}\left(\mathbf{R}_2\right)$.

The one-electron density matrix of $\Phi$ is

$$\gamma_s(\mathbf{x}, \mathbf{x}') = \left\langle \Phi \left| \sum_i^{2N+1} \hat{\gamma}(i) \right| \Phi \right\rangle,$$

where

$$\hat{\gamma}(i) = \delta\left(\mathbf{x} - \mathbf{x}_i\right)\delta\left(\mathbf{x}' - \mathbf{x}_i'\right).$$

We have

$$\begin{aligned}\gamma_s(\mathbf{x}, \mathbf{x}') = (&\gamma^0_{s\mathbf{R}_1}(N) + \gamma^{n_s}_{s\mathbf{R}_1}(N+1) + \gamma^0_{s\mathbf{R}_2}(N) \\ &+ \gamma^{n_s}_{s\mathbf{R}_2}(N+1))/2 + C_1(\mathbf{x}, \mathbf{x}'),\end{aligned} \tag{4}$$

where the direct terms $\gamma^0_{s\mathbf{R}_1}(N)$ and $\gamma^{n_s}_{s\mathbf{R}_1}(N+1)$, coming from $\langle \Phi_\alpha \left| \hat{\gamma}_s(\mathbf{x},\mathbf{x}') \right| \Phi_\alpha \rangle$ and $\langle \Phi_\beta \left| \hat{\gamma}_s(\mathbf{x},\mathbf{x}') \right| \Phi_\beta \rangle$, are the density matrices of $\Phi^0_N(\mathbf{R}_1)$ and $\Phi^{n_s}_{N+1}(\mathbf{R}_1)$ respectively. The cross term is

$$C_1(\mathbf{x},\mathbf{x}') = \frac{1}{2}\left(\left\langle \Phi_\alpha \left| \sum_i^{2N+1} \hat{\gamma}(i) \right| \Phi_\beta \right\rangle + c.c.\right).$$

We use $u_1 u_2 ... u_N$ to denote the one electron orbitals for $\Phi^0_N(\mathbf{R}_1)$ ,$u_{N+1} u_{N+2} ... u_{2N+1}$ for $\Phi^{n_s}_{N+1}(\mathbf{R}_2)$, $v_1 v_2 ... v_{N+1}$ for $\Phi^{n_s}_{N+1}(\mathbf{R}_1)$, and $v_{N+2} v_{N+2} ... v_{2N+1}$ for $\Phi^0_N(\mathbf{R}_2)$ . Based on Lowdin's general formulae for nonorthogonal orbitals [1], the cross term $\langle \Phi_\beta \left| \hat{\gamma}_s(\mathbf{x},\mathbf{x}') \right| \Phi_\alpha \rangle$ is given by

$$\left\langle \Phi_\beta \left| \sum_i^{2N+1} \hat{\gamma}(i) \right| \Phi_\alpha \right\rangle = \sum_{i,j=1} \langle v_i | \hat{\gamma} | u_j \rangle \, D(i|j),$$

where $D(i|j)$ is the algebraic complement,

$$D(i|j) = (-1)^{i+j} M(i|j),$$

where $M(i|j)$ is the minor of the overlap matrix $\mathbf{S}$, with $S_{ij} = \langle v_i | u_j \rangle$. The wavefunction overlap is given by the determinant of $\mathbf{S}$ [1].

$$\langle \Phi_\beta | \Phi_\alpha \rangle = \det \mathbf{S} = 0,$$

which is due to the fact that $\Phi^0_N(\mathbf{R}_1)$ is strongly orthogonal to $\Phi^{n_s}_{N+1}(\mathbf{R}_2)$, and $\Phi^{n_s}_{N+1}(\mathbf{R}_1)$ to $\Phi^0_N(\mathbf{R}_2)$. This can also be understood from the structure of $\mathbf{S}$ as described in Table I A. For the first $N+1$ rows of $\mathbf{S}$, each row has the $N$ nonzero elements that are the first $N$ elements . One can carry our row elementary operations within the the first $N+1$ rows and generate a row of all zero elements. In other words, the first $N+1$ row vectors are linearly dependent. Therefore det$\mathbf{S}$= 0. Similarly, the last $(N+1)$ column vectors of the $\mathbf{S}$ matrix are also linear dependent, because each column vector has the $N$ nonzero elements that are the last $N$ elements.

For a minor $M(i|j)$ to be nonzero: $i$ has to be in the first $N+1$ rows, and j has to be in the last $N+1$ column. That is

$$\begin{aligned}\left\langle \Phi_\beta \left| \sum_i^{2N+1} \hat{\gamma}(i) \right| \Phi_\alpha \right\rangle &= \sum_{1\le i\le N+1, N+1\le j\le 2N+1} \langle v_i | \hat{\gamma} | u_j \rangle \, D(i|j) \\ &= \sum_{1\le i\le N+1, N+1\le j\le 2N+1} {v_i}^*(\mathbf{x}) u_j(\mathbf{x}') D(i|j)\end{aligned}$$

TABLE I. The structure of the overlap matrix $\mathbf{S}$

| | | $\Phi_N^0(\mathbf{R}_1)$ | | | | $\Phi_{N+1}^{n_s}(\mathbf{R}_2)$ | | | |
|---|---|---|---|---|---|---|---|---|---|
| | | $u_1$ | $u_2$ | ... | $u_N$ | $u_{N+1}$ | $u_{N+2}$ | ... | $u_{2N+1}$ |
| $\Phi_{N+1}^{n_s}(\mathbf{R}_1)$ | $v_1$ | $\langle v_1\|u_1\rangle$ | $\langle v_1\|u_2\rangle$ | ... | $\langle v_1\|u_N\rangle$ | 0 | 0 | 0 | 0 |
| | $v_2$ | $\langle v_2\|u_1\rangle$ | $\langle v_2\|u_2\rangle$ | | $\langle v_2\|u_N\rangle$ | 0 | 0 | 0 | 0 |
| | ... | ... | ... | ... | ... | 0 | 0 | 0 | 0 |
| | $v_{N+1}$ | $\langle v_{N+1}\|u_1\rangle$ | $\langle v_{N+1}\|u_2\rangle$ | ... | $\langle v_{N+1}\|u_N\rangle$ | 0 | 0 | 0 | 0 |
| $\Phi_N^0(\mathbf{R}_2)$ | $v_{N+2}$ | 0 | 0 | 0 | 0 | $\langle v_{N+2}\|u_{N+1}\rangle$ | $\langle v_{N+2}\|u_{N+2}\rangle$ | ... | $\langle v_{N+2}\|u_{2N+1}\rangle$ |
| | $v_{N+3}$ | 0 | 0 | 0 | 0 | $\langle v_{N+3}\|u_{N+1}\rangle$ | $\langle v_{N+3}\|u_{N+2}\rangle$ | ... | $\langle v_{N+3}\|u_{2N+1}\rangle$ |
| | ... | 0 | 0 | 0 | 0 | ... | ... | ... | ... |
| | $v_{2N+1}$ | 0 | 0 | 0 | 0 | $\langle v_{N+2}\|u_{N+1}\rangle$ | $\langle v_{N+2}\|u_{N+2}\rangle$ | ... | $\langle v_{N+2}\|u_{2N+1}\rangle$ |

For $1 \le i \le N, N+1 \le 2N+1$, $v_i{}^*(\mathbf{x})u_j(\mathbf{x}') = 0$, for all $|\mathbf{r}-\mathbf{r}'| < \infty$,because $v_i{}^*(\mathbf{x})$ is from $\Phi_{N+1}^{n_s}(\mathbf{R}_1)$ and $u_j(\mathbf{x}')$ from $\Phi_{N+1}^{n_s}(\mathbf{R}_2)$ and $|\mathbf{R}_1 - \mathbf{R}_2| \to \infty$. Therefore we show that

$$C_1(\mathbf{x},\mathbf{x}') = \begin{cases} 0, & |\mathbf{r}-\mathbf{r}'| < \infty \\ \neq 0, & |\mathbf{r}-\mathbf{r}'| \to \infty. \end{cases}$$

### B. All fractions

The extension to all fractions is similar. We just need to extend the overlap matrix to include all locations, $\mathbf{R}_1, \mathbf{R}_2, ...\mathbf{R}_q$. The only nonzero contribution to the cross term $C_2(\mathbf{x},\mathbf{x}')$ of Eq.(15) of the main text, are from $v_i{}^*(\mathbf{x})u_j(\mathbf{x}')D(i|j)$, when $v_i{}^*(\mathbf{x})$ is from $\Phi_{N+1}^{n_s}\left(\mathbf{R}_{p_1}\right)$ and $u_j(\mathbf{x}')$ from $\Phi_{N+1}^{n_s}\left(\mathbf{R}_{p_2}\right)$. Thus

$$C_2(\mathbf{x},\mathbf{x}') = \begin{cases} 0, & |\mathbf{r}-\mathbf{r}'| < \infty \\ \neq 0, & |\mathbf{r}-\mathbf{r}'| \to \infty. \end{cases}$$

### C. The contribution of the cross term to the total energy

We here examine the contribution of 1-particle density matrix of entangled states to the total energy. It is sufficient to consider the half integer case. We have two identical

subsystems, one at $\mathbf{R}_1$ and the other at $\mathbf{R}_2$, $|\mathbf{R}_1 - \mathbf{R}_2| \to \infty$. The 1-particle density matrix of the noninteracting wavefunction $\Phi$, Eq. (3) is

$$\gamma_s(\mathbf{x}, \mathbf{x}') = (\gamma^0_{s\mathbf{R}_1}(N) + \gamma^{n_s}_{s\mathbf{R}_1}(N+1) + \gamma^0_{s\mathbf{R}_2}(N) \\ + \gamma^{n_s}_{s\mathbf{R}_2}(N+1))/2 + C_1(\mathbf{x}, \mathbf{x}') \tag{5}$$

For any $|\mathbf{r} - \mathbf{r}'| < \infty$, $\gamma_s(\mathbf{x}, \mathbf{x}')$ is separable as the sum of two subsystem density matrices,

$$\gamma_s(\mathbf{x}, \mathbf{x}') = \frac{1}{2}(\gamma^0_{s\mathbf{R}_1}(N) + \gamma^{n_s}_{s\mathbf{R}_1}(N+1)) + \frac{1}{2}(\gamma^0_{s\mathbf{R}_2}(N) + \gamma^{n_s}_{s\mathbf{R}_2}(N+1))$$

The cross term $C_1(\mathbf{x}, \mathbf{x}')$ have nonzero values only when $|\mathbf{r} - \mathbf{r}'| \to \infty$ and as such it cannot make finite contribution to the total energy; If $C_1(\mathbf{x}, \mathbf{x}')$ contributes to total energy for $|\mathbf{r} - \mathbf{r}'| \to \infty$, one would expect the resulting total energy not to be a finite number. Similar conclusion was reached for the physical density matrices [2].

Thus we have

$$E_v[\gamma_s(\mathbf{x}, \mathbf{x}')] \\ = E_v[\frac{1}{2}(\gamma^0_{s\mathbf{R}_1}(N) + \gamma^{n_s}_{s\mathbf{R}_1}(N+1)) + \frac{1}{2}(\gamma^0_{s\mathbf{R}_2}(N) + \gamma^{n_s}_{s\mathbf{R}_2}(N+1))], \tag{6}$$

which is used in the main text before Eq. (9).

## II. EXCITED-STATE CHEMICAL CONCEPTS

The present introduction of fractional charges and excited-state chemical potentials also allows us to explore the chemical concepts for excited states, leading to excited state electronegativity, hardness, and fukui functions, extending corresponding ground-state concepts [3–5]. These excited-state chemical concepts can be useful for describing chemical reactivity in excited states, just as the ground-state concepts [6].

In contrast to the ground-state theory, where the fractional particle number $\mathcal{N}$is sufficient to characterize the chemical changes between ground states. In excited-state theory, there are many possibilities for changing the fractional particle number $\mathcal{N}$ and we have to specify the particular process from one state to another. Therefore, in analogy to the ground-state electronegativity [5], we define the $N$-electron *excited-state eletronegativity* as the negative of the corresponding chemical potentials: on the electron addition side, it is

$$\chi^{+}_{n_s m_s} = -\mu^{+}_{n_s m_s} = E^{n}_{v}(N) - E^{m}_{v}(N+1), \tag{7}$$

and on the electron removal side, it is

$$\chi^{-}_{n_s l_s} = -\mu^{-}_{n_s l_s} = E^{l}_{v}(N-1) - E^{n}_{v}(N), \tag{8}$$

where we have used the exact chemical potential expressions proved in the main text. Thus $\chi^{+}_{n_s m_s}$ is the excited state IP and $\chi^{-}_{n_s l_s}$ is the excited-state EA. Then the excited-state Mulliken definition of the electronegativity is the average

$$\chi^{M}_{l_s n_s m_s} = \frac{1}{2}(\chi^{+}_{n_s m_s} + \chi^{-}_{n_s l_s}), \tag{9}$$

extending the ground state results [5]. But now it has three indexes for three excited states involved.

Similarly, we define the *excited-state chemical hardness*, as half of the discontinuity in the electronegativity from two sides of the integer $N$ namely

$$\eta^{M}_{l_s n_s m_s} = \frac{1}{2}(\chi^{-}_{n_s l_s} - \chi^{+}_{n_s m_s}), \tag{10}$$

in analogy to the ground state *chemical hardness* [4].

Following the ground-state theory [3], we define excited-state fukui function as the derivative of the electron density with respect to the fractional particle number $\mathcal{N}$. On the electron

addition side, $\mathcal{N} = (1-\delta)N + \delta(N+1) = N + \delta$, $\gamma_s = (1-\delta)\gamma_s^{n_s}(N) + \delta\gamma_s^{m_s}(N+1)$, the density is $\rho^+_{n_s m_s}(\mathbf{r}) = (1-\delta)\rho^{n_s}(\mathbf{r}, N) + \delta\rho^{m_s}(\mathbf{r}, N+1)$, and the fukui function is

$$\begin{aligned} f^+_{n_s,m_s}(\mathbf{r}) &= \left(\frac{\partial \rho^+_{n_s m_s}(\mathbf{r})}{\partial \mathcal{N}}\right)_v \\ &= \rho^{m_s}(\mathbf{r}, N+1) - \rho^{n_s}(\mathbf{r}, N). \end{aligned} \tag{11}$$

And on the electron removal side, $\mathcal{N} = (1-\delta)N + \delta(N-1) = N - \delta$, $\gamma_s = (1-\delta)\gamma_s^{n_s}(N) + \delta\gamma_s^{l_s}(N-1)$, the density is $\rho^-_{n_s l_s}(\mathbf{r}) = (1-\delta)\rho^{n_s}(\mathbf{r}, N) + \delta\rho^{l_s}(\mathbf{r}, N-1)$, and the fukui function is

$$\begin{aligned} f^-_{n_s,l_s}(\mathbf{r}) &= \left(\frac{\partial \rho^-_{n_s l_s}(\mathbf{r})}{\partial \mathcal{N}}\right)_v \\ &= \rho^{n_s}(\mathbf{r}, N) - \rho^{l_s}(\mathbf{r}, N-1). \end{aligned} \tag{12}$$

All these excited-state concepts are direct extensions from the ground-state definitions. Apart from the analogy, how they characterize the chemical properties of excited states should be further explored.

## III. COMPUTATIONAL DETAILS AND RESULTS FOR EXCITATION ENERGIES OF FRACTIONAL CHARGE SYSTEMS

In the following text, three conventional DFAs, LDA[7], BLYP[8, 9] and B3LYP[8–10] were tested for the $\Delta SCF$ approach, and the calculations were performed with the QM4D package[11]; CCSD(T) and EOM-CCSD calculations were performed with PySCF package[12, 13]. $\Delta SCF$ calculations were performed based on the maximum overlap method (MOM)[14]. All data presented in this document were based on spin-unrestricted calculations, and the SCF calculation for fractional charge systems are based on Ref [15]. The SCF iterations did not converge for some fractionally charged systems, and they are labeled with N/A (not applicable) in the following text.

### A. OH radical electron addition and removal

The total energies for fractionally charged systems during the electron removal from the ground state and the excited state $((1s)^2(2s)^2(\sigma)(n)^3(\sigma^*))$ of the OH radical (N=9) to the ground state and the excited state $((1s)^2(2s)^2(\sigma)(n)^3)$ of $OH^+$ (N = 8), and also the electron addition to the ground state and the excited state $((1s)^2(2s)^2(\sigma)^2(n)^3(\sigma^*))$ of $OH^-$ (N=10) were calculated for three conventional DFAs (LDA, BLYP and B3LYP). LDA and B3LYP total energies were corrected with LOSC2[16]. The BLYP total energy were corrected based on the lrLOSC[17–19]. Becuse of the effect from higher order expansion of DFA total energy, some valence orbitals have unphysical lrLOSC curvatures. [20] In this work, we are replacing those unphysical curvatures by the LOSC2 [16] curvatures. All calculations were based on the ground state geometry and the length of the O-H bond is 0.9827 Å. The basis set def2-TZVPD[21, 22] was used for all calculations in this section.

#### 1. *The molecular orbital diagram for the ground and excited states of OH radical/ion*

The electron occupation details for the states of interest are given in the following MO diagrams. The 1s and 2s orbitals come from the 1s and 2s atomic orbitals of the oxygen atom, and $n$ are two non-bonding orbitals that come from the 2p atomic orbitals of the oxygen atom. The $\sigma$ and $\sigma^*$ are the $\sigma$ bonding or anti-bonding orbitals. Notice that the orbital

energies from different spins can be different since we used spin-unrestricted calculations, but they are placed at the same energy levels for clarity.

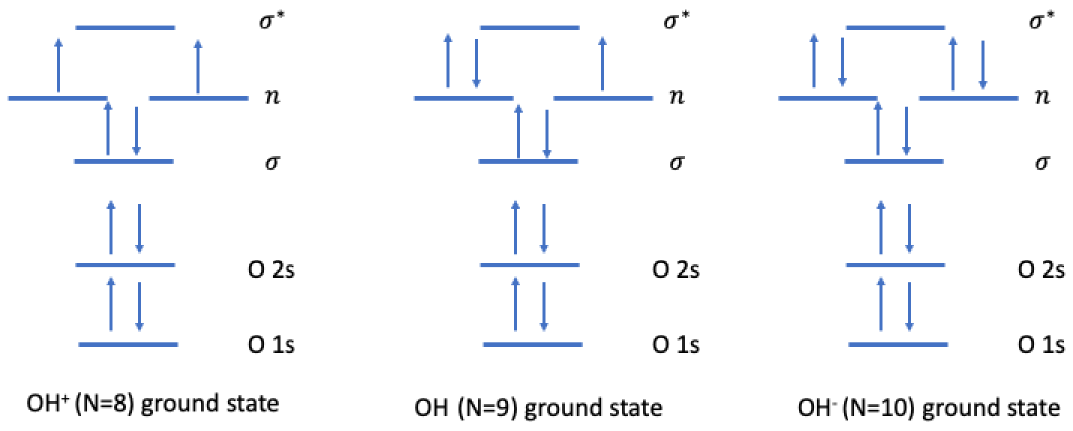


FIG. 1. Ground-state electron occupation details for $OH^+$, OH and $OH^-$

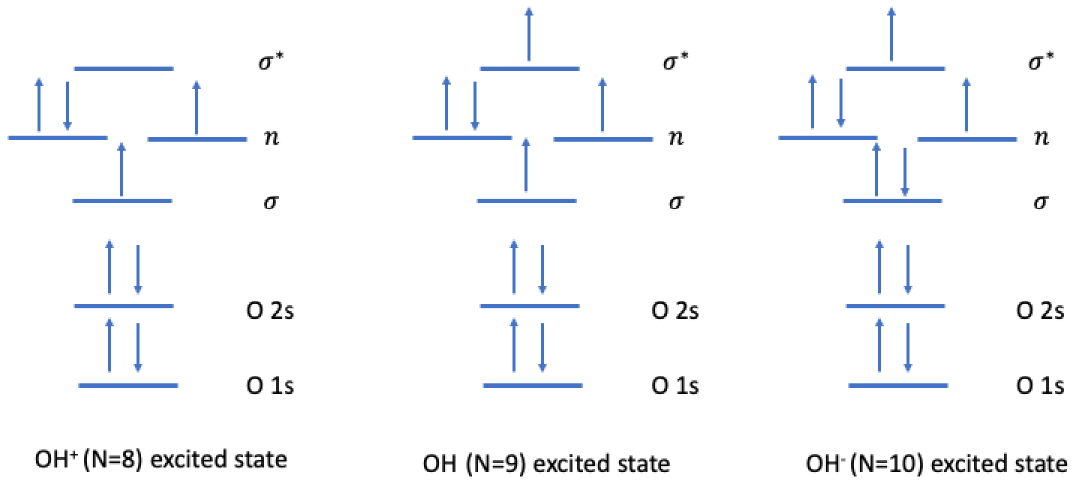


FIG. 2. Excited-state electron occupation details for $OH^+$, OH and $OH^-$

### *2. Ground state electron addition and removal*

TABLE II. The BLYP total energy ($E_h$) for the electron removal from OH radical (N=9) ground state to the $OH^+$ (N=8) ground state and also the electron addition to the $OH^-$ (N=10) ground state. LOSC corrections are based lrLOSC[17–19].

| Number of electrons | BLYP total energy | LOSC-BLYP total energy | Exact linear condition |
|---|---|---|---|
| 8.0 | -75.270360 | -75.270360 | -75.270360 |
| 8.1 | -75.339248 | -75.317118 | -75.319163 |
| 8.2 | -75.403671 | -75.364582 | -75.367965 |
| 8.3 | -75.463591 | -75.412658 | -75.416768 |
| 8.4 | -75.518997 | -75.461248 | -75.465570 |
| 8.5 | -75.569902 | -75.510258 | -75.514373 |
| 8.6 | -75.616335 | -75.559593 | -75.563175 |
| 8.7 | -75.658339 | -75.609163 | -75.611978 |
| 8.8 | -75.695967 | -75.658878 | -75.660780 |
| 8.9 | -75.729289 | -75.708647 | -75.709583 |
| 9.0 | -75.758385 | -75.758385 | -75.758385 |
| 9.1 | -75.780600 | -75.761159 | -75.765599 |
| 9.2 | -75.799285 | -75.765040 | -75.772814 |
| 9.3 | -75.814475 | -75.769988 | -75.780028 |
| 9.4 | -75.826233 | -75.775961 | -75.787242 |
| 9.5 | -75.834641 | -75.782908 | -75.794456 |
| 9.6 | -75.839801 | -75.790778 | -75.801671 |
| 9.7 | -75.841831 | -75.799515 | -75.808885 |
| 9.8 | -75.840864 | -75.809071 | -75.816099 |
| 9.9 | -75.837044 | -75.819410 | -75.823314 |
| 10.0 | -75.830528 | -75.830528 | -75.830528 |

TABLE III. The B3LYP total energy ($E_h$) for the electron removal from OH radical (N=9) ground state to the $OH^+$ (N=8) ground state and also the electron addition to the $OH^-$ (N=10) ground state. LOSC corrections are based on LOSC2 [16].

| Number of electrons | B3LYP total energy | LOSC-B3LYP total energy | Exact linearity condition |
|---|---|---|---|
| 8.0 | -75.282138 | -75.282138 | -75.282138 |
| 8.1 | -75.345655 | -75.328553 | -75.331014 |
| 8.2 | -75.411746 | -75.380352 | -75.379891 |
| 8.3 | -75.468379 | -75.428071 | -75.428767 |
| 8.4 | -75.521728 | -75.476345 | -75.477643 |
| 8.5 | -75.571804 | -75.525138 | -75.526520 |
| 8.6 | -75.618631 | -75.574418 | -75.575396 |
| 8.7 | -75.662240 | -75.624159 | -75.624272 |
| 8.8 | -75.702669 | -75.674344 | -75.673148 |
| 8.9 | -75.739965 | -75.724965 | -75.722025 |
| 9.0 | -75.770901 | -75.770901 | -75.770901 |
| 9.1 | -75.788102 | -75.773488 | -75.777679 |
| 9.2 | -75.802822 | -75.776984 | -75.784458 |
| 9.3 | -75.815098 | -75.781381 | -75.791236 |
| 9.4 | -75.824982 | -75.786672 | -75.798015 |
| 9.5 | -75.832539 | -75.792855 | -75.804793 |
| 9.6 | -75.837845 | -75.799944 | -75.811571 |
| 9.7 | -75.840995 | -75.807972 | -75.818350 |
| 9.8 | -75.842095 | -75.817007 | -75.825128 |
| 9.9 | -75.841273 | -75.827173 | -75.831906 |
| 10.0 | -75.838685 | -75.838685 | -75.838685 |

TABLE IV. The LDA total energy ($E_h$) for the electron removal from OH radical (N=9) ground state to the $OH^+$ (N=8) ground state and also the electron addition to the $OH^-$ (N=10) ground state. LOSC corrections are based on LOSC2 [16].

| Number of electrons | LDA total energy | LOSC-LDA total energy | Exact linearity condition |
|---|---|---|---|
| 8.0 | -74.707282 | -74.707282 | -74.707282 |
| 8.1 | -74.777668 | -74.755372 | -74.756824 |
| 8.2 | -74.843359 | -74.804056 | -74.806366 |
| 8.3 | -74.904349 | -74.853225 | -74.855907 |
| 8.4 | -74.960653 | -74.902776 | -74.905449 |
| 8.5 | -75.012300 | -74.952607 | -74.954991 |
| 8.6 | -75.059336 | -75.002625 | -75.004533 |
| 8.7 | -75.101819 | -75.052735 | -75.054075 |
| 8.8 | -75.139818 | -75.102846 | -75.103616 |
| 8.9 | -75.173415 | -75.152865 | -75.153158 |
| 9.0 | -75.202700 | -75.202700 | -75.202700 |
| 9.1 | -75.227356 | -75.207436 | -75.211413 |
| 9.2 | -75.248216 | -75.213219 | -75.220126 |
| 9.3 | -75.265340 | -75.219986 | -75.228839 |
| 9.4 | N/A | N/A | -75.237552 |
| 9.5 | N/A | N/A | -75.246265 |
| 9.6 | N/A | N/A | -75.254978 |
| 9.7 | N/A | N/A | -75.263691 |
| 9.8 | N/A | N/A | -75.272404 |
| 9.9 | -75.291190 | -75.288575 | -75.281117 |
| 10.0 | -75.289830 | -75.289830 | -75.289830 |

### 3. *Excited state to ground state electron addition and removal*

TABLE V. The BLYP total energy ($E_h$) the electron removal from the ground state of the OH radical (N=9) to the $OH^+$ (N=8) excited state ($(1s)^2(2s)^2(\sigma)(n)^3$) and also the electron addition to the $OH^-$ (N=10) excited state ($(1s)^2(2s)^2(\sigma)^2(n)^3(\sigma^*)$). LOSC corrections are based lrLOSC[17–19].

| Number of electrons | BLYP total energy | LOSC-BLYP total energy | Exact linear condition |
|---|---|---|---|
| 8.0 | -75.138188 | -75.138188 | -75.138188 |
| 8.1 | -75.219709 | -75.199207 | -75.200207 |
| 8.2 | -75.297040 | -75.260807 | -75.262227 |
| 8.3 | -75.370000 | -75.322753 | -75.324246 |
| 8.4 | -75.438575 | -75.384954 | -75.386266 |
| 8.5 | -75.502755 | -75.447303 | -75.448286 |
| 8.6 | -75.562549 | -75.509710 | -75.510305 |
| 8.7 | -75.617970 | -75.572088 | -75.572325 |
| 8.8 | -75.669055 | -75.634368 | -75.634344 |
| 8.9 | -75.715843 | -75.696485 | -75.696364 |
| 9.0 | -75.758384 | -75.758384 | -75.758384 |
| 9.1 | -75.760139 | -75.752574 | -75.752690 |
| 9.2 | -75.760430 | -75.747182 | -75.746996 |
| 9.3 | -75.759093 | -75.742014 | -75.741302 |
| 9.4 | -75.756048 | -75.736916 | -75.735608 |
| 9.5 | -75.751263 | -75.731750 | -75.729914 |
| 9.6 | -75.744732 | -75.726406 | -75.724220 |
| 9.7 | -75.736464 | -75.720780 | -75.718526 |
| 9.8 | -75.726479 | -75.714790 | -75.712832 |
| 9.9 | -75.714798 | -75.708361 | -75.707138 |
| 10.0 | -75.701444 | -75.701444 | -75.701444 |

TABLE VI. The LDA total energy ($E_h$) the electron removal from the ground state of the OH radical (N=9) to the $OH^+$ (N=8) excited state ($(1s)^2(2s)^2(\sigma)(n)^3$) and also the electron addition to the $OH^-$ (N=10) excited state ($(1s)^2(2s)^2(\sigma)^2(n)^3(\sigma^*)$). LOSC corrections are based on LOSC2 [16].

| Number of electrons | LDA total energy | LOSC-LDA total energy | Exact linear condition |
|---|---|---|---|
| 8.0 | -74.576100 | -74.576100 | -74.576100 |
| 8.1 | -74.659011 | -74.638310 | -74.638760 |
| 8.2 | -74.737428 | -74.700892 | -74.701420 |
| 8.3 | -74.811326 | -74.763737 | -74.764080 |
| 8.4 | -74.880688 | -74.826729 | -74.826740 |
| 8.5 | -74.945517 | -74.889764 | -74.889400 |
| 8.6 | -75.005829 | -74.952750 | -74.952060 |
| 8.7 | -75.061656 | -75.015606 | -75.014720 |
| 8.8 | -75.113040 | -75.078257 | -75.077380 |
| 8.9 | -75.160034 | -75.140640 | -75.140040 |
| 9.0 | -75.202700 | -75.202700 | -75.202700 |
| 9.1 | -75.204452 | -75.196755 | -75.197584 |
| 9.2 | -75.205071 | -75.191678 | -75.192467 |
| 9.3 | -75.204204 | -75.187014 | -75.187351 |
| 9.4 | -75.201720 | -75.182519 | -75.182235 |
| 9.5 | -75.197565 | -75.178020 | -75.177119 |
| 9.6 | -75.191721 | -75.173381 | -75.172002 |
| 9.7 | -75.184187 | -75.168492 | -75.166886 |
| 9.8 | -75.174969 | -75.163265 | -75.161770 |
| 9.9 | -75.164082 | -75.157632 | -75.156654 |
| 10.0 | -75.151537 | -75.151537 | -75.151537 |

TABLE VII. The B3LYP total energy ($E_h$) for the electron removal from the ground state of the OH radical (N=9) to the $OH^+$ (N=8) excited state ($(1s)^2(2s)^2(\sigma)(n)^3$) and also the electron addition to the $OH^-$ (N=10) excited state ($(1s)^2(2s)^2(\sigma)^2(n)^3(\sigma^*)$). LOSC corrections are based on LOSC2 [16].

| Number of electrons | B3LYP total energy | LOSC-B3LYP total energy | Exact linearity condition |
|---|---|---|---|
| 8.0 | -75.149100 | -75.149100 | -75.149100 |
| 8.1 | N/A | N/A | -75.211280 |
| 8.2 | -75.298964 | -75.270839 | -75.273460 |
| 8.3 | -75.369310 | -75.332536 | -75.335640 |
| 8.4 | -75.436393 | -75.394528 | -75.397820 |
| 8.5 | -75.500208 | -75.456769 | -75.460001 |
| 8.6 | -75.560774 | -75.519235 | -75.522181 |
| 8.7 | -75.618103 | -75.581895 | -75.584361 |
| 8.8 | -75.672208 | -75.644724 | -75.646541 |
| 8.9 | -75.723127 | -75.707722 | -75.708721 |
| 9.0 | -75.770901 | -75.770901 | -75.770901 |
| 9.1 | -75.771174 | -75.765331 | -75.765520 |
| 9.2 | -75.770427 | -75.760140 | -75.760139 |
| 9.3 | -75.768472 | -75.755138 | -75.754758 |
| 9.4 | -75.765219 | -75.750200 | -75.749377 |
| 9.5 | -75.760621 | -75.745220 | -75.743996 |
| 9.6 | -75.754657 | -75.740111 | -75.738615 |
| 9.7 | -75.747319 | -75.734801 | -75.733233 |
| 9.8 | -75.738608 | -75.729227 | -75.727852 |
| 9.9 | -75.728530 | -75.723338 | -75.722471 |
| 10.0 | -75.717090 | -75.717090 | -75.717090 |

### 4. *Excited state to excited state electron addition and removal*

TABLE VIII. The BLYP total energy ($E_h$) for the electron removal from the ground state and the excited state ($(1s)^2(2s)^2(\sigma)(n)^3(\sigma^*)$) of the OH radical (N=9) to the excited state ($(1s)^2(2s)^2(\sigma)(n)^3$) of the $OH^+$ (N=8) and also the electron addition to the excited state ($(1s)^2(2s)^2(\sigma)^2(n)^3(\sigma^*)$) of the $OH^-$ (N=10). LOSC corrections are based on lrLOSC[17–19].

| Number of electrons | BLYP total energy | LOSC-BLYP total energy | Exact linearity condition |
|---|---|---|---|
| 8.0 | -75.138188 | -75.138188 | -75.138188 |
| 8.1 | -75.172327 | -75.160249 | -75.159969 |
| 8.2 | -75.203803 | -75.181211 | -75.181750 |
| 8.3 | -75.232463 | -75.202408 | -75.203531 |
| 8.4 | -75.258265 | -75.224141 | -75.225312 |
| 8.5 | -75.281202 | -75.246336 | -75.247093 |
| 8.6 | -75.301381 | -75.268859 | -75.268874 |
| 8.7 | -75.318848 | -75.291398 | -75.290656 |
| 8.8 | -75.333701 | -75.313644 | -75.312437 |
| 8.9 | -75.346033 | -75.335260 | -75.334218 |
| 9.0 | -75.355999 | -75.355999 | -75.355999 |
| 9.1 | -75.405290 | -75.391185 | -75.390543 |
| 9.2 | -75.451450 | -75.425773 | -75.425088 |
| 9.3 | -75.494403 | -75.460134 | -75.459632 |
| 9.4 | -75.534092 | -75.494369 | -75.494177 |
| 9.5 | -75.570473 | -75.528572 | -75.528721 |
| 9.6 | -75.603503 | -75.562815 | -75.563265 |
| 9.7 | -75.633143 | -75.597196 | -75.597810 |
| 9.8 | -75.659361 | -75.631778 | -75.632354 |
| 9.9 | -75.682128 | -75.666553 | -75.666899 |
| 10.0 | -75.701443 | -75.701443 | -75.701443 |

*5. Plot for the fractional charged system total energies with respect to the number of electrons.*

In this section, the system total energies ($E_h$) for the fractional charged systems carried with respect to the number of electrons were plotted in this section based on the data presented in previous texts. The total energy plot carried out with the BLYP functional is presented in the main text, and the plots carried out with the LDA (FIG. 3.) and B3LYP (FIG. 4.) functionals are presented in this document. The LDA plot (FIG. 3.) is based on Table IV and Table VI, and the B3LYP plot (FIG. 4.) is based on Table III and Table VII.

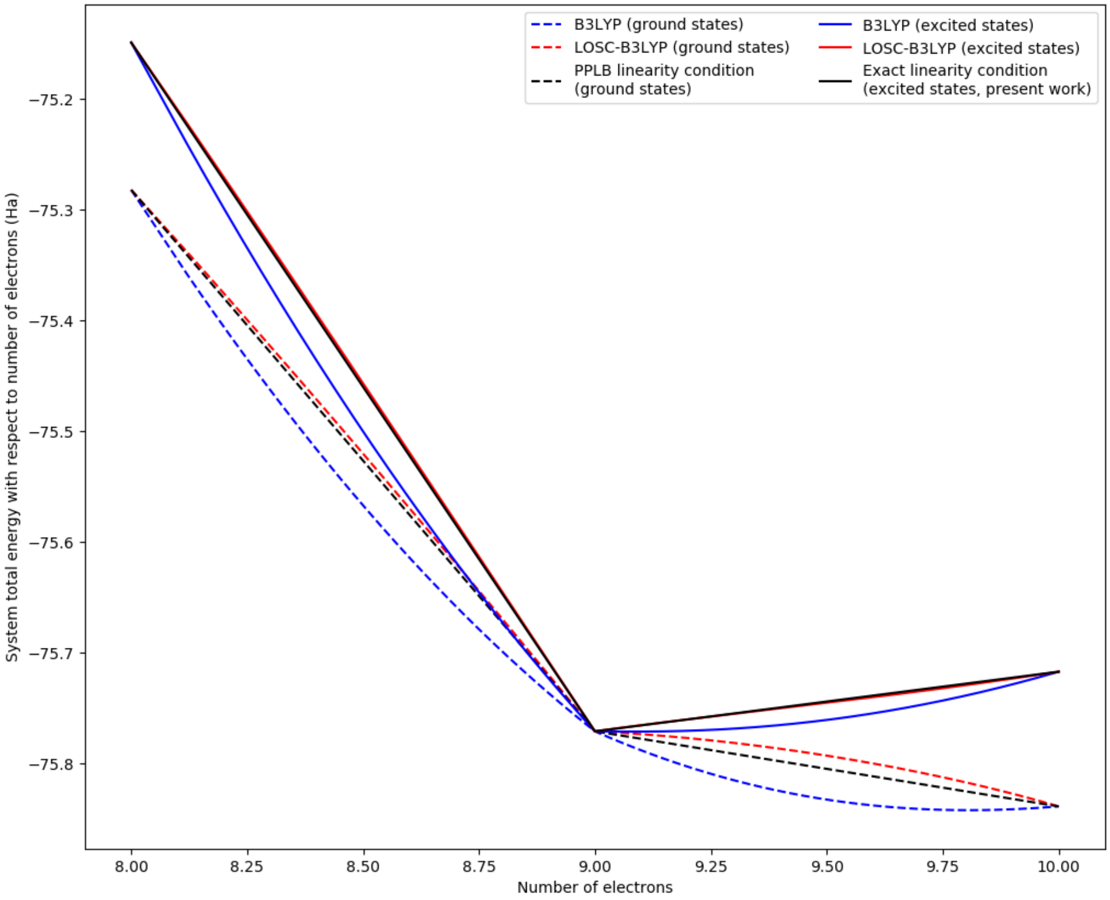


FIG. 3. The total energies of fractional charges from the ground state of the OH molecule (N = 9) to the ground and the (n $\rightarrow \sigma^*$) excited state of $OH^-$ (N = 10) and also to the ground and the ($\sigma \rightarrow$ n) excited state of $OH^+$ (N = 8). All calculations were carried out with the B3LYP functional. LOSC corrections are based on LOSC2 [16].

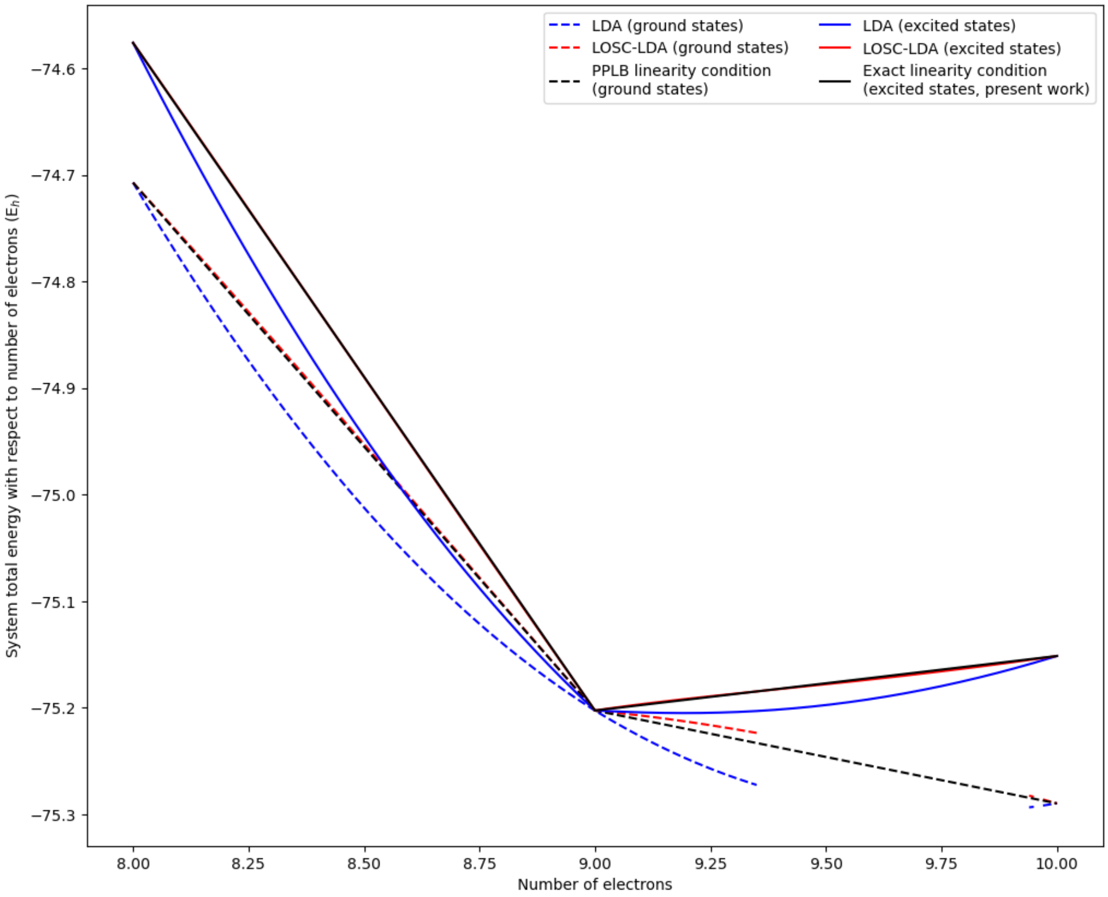


FIG. 4. The total energies of fractional charges from the ground state of the OH molecule (N = 9) to the ground and the (n $\rightarrow \sigma^*$) excited state of $OH^-$ (N = 10) and also to the ground and the ($\sigma \rightarrow$ n) excited state of $OH^+$ (N = 8). All calculations were carried out with the LDA functional. Discontinuities on the electron affinity side result from the SCF convergence issue encountered for certain fractionally charged systems. LOSC corrections arre based on LOSC2[16].

### B. Li atom electron addition and removal

The second system of interest is the electron removal from the ground state of Li atom (N =3) to the ground and excited states ($(1s)(2s)$) of $Li^+$ (N=2) and also the electron addition to the $Li^-$ (N=4) ground and excited states ($(1s)^2(2s)(2p)$). Def2-TZVPD was used as the basis set for all calculations in this section. All LOSC calculations in this section were carrried out using LOSC2[16].

### 1. *Ground state electron addition and removal*

TABLE IX. Total energies ($E_h$) for the electron removal from the ground state of Li atom (N=3) to the ground state of $Li^+$ (N=2) cation and also the electron addition to the ground state of $Li^-$ (N=4) anion. LOSC corrections are based on LOSC2 [16].

| Number of electrons | BLYP total energy | LOSC-BLYP total energy | Exact linearity condition |
|---|---|---|---|
| 2.0 | -7.279287 | -7.279287 | -7.279287 |
| 2.1 | -7.307128 | -7.299229 | -7.299603 |
| 2.2 | -7.333782 | -7.319928 | -7.319918 |
| 2.3 | -7.358824 | -7.340869 | -7.340233 |
| 2.4 | -7.382102 | -7.361845 | -7.360549 |
| 2.5 | -7.403538 | -7.382721 | -7.380864 |
| 2.6 | -7.423094 | -7.403393 | -7.401180 |
| 2.7 | -7.440753 | -7.423774 | -7.421495 |
| 2.8 | -7.456520 | -7.443788 | -7.441811 |
| 2.9 | -7.470408 | -7.463365 | -7.462126 |
| 3.0 | -7.482442 | -7.482442 | -7.482442 |
| 3.1 | -7.489251 | -7.482760 | -7.483263 |
| 3.2 | -7.495141 | -7.483803 | -7.484085 |
| 3.3 | -7.499673 | -7.485039 | -7.484906 |
| 3.4 | -7.502764 | -7.486306 | -7.485728 |
| 3.5 | -7.504392 | -7.487511 | -7.486549 |
| 3.6 | -7.504555 | -7.488589 | -7.487370 |
| 3.7 | -7.503255 | -7.489485 | -7.488192 |
| 3.8 | -7.500500 | -7.490155 | -7.489013 |
| 3.9 | -7.496297 | -7.490557 | -7.489835 |
| 4.0 | -7.490656 | -7.490656 | -7.490656 |

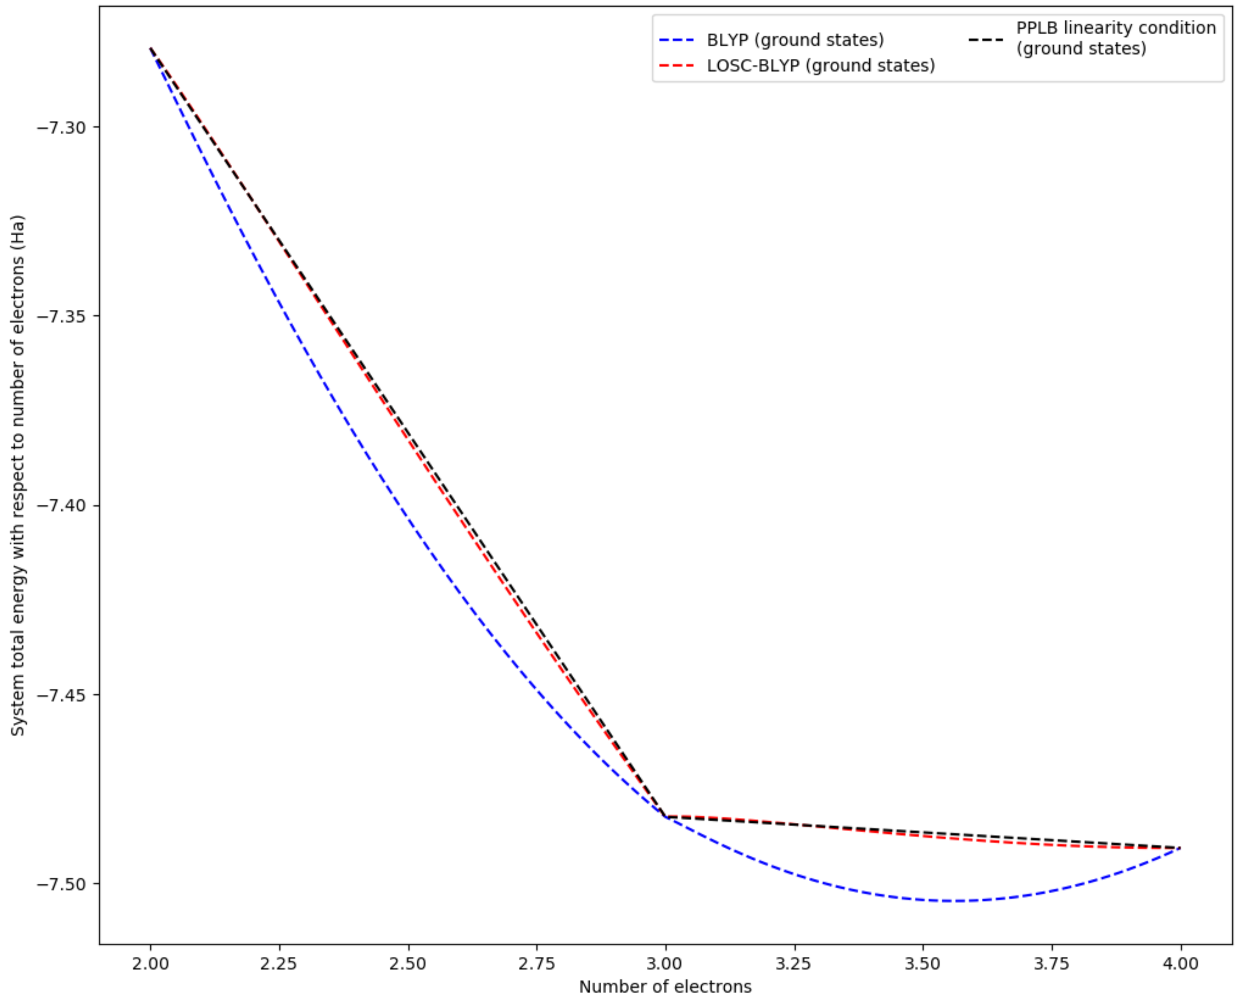


FIG. 5. The total energies ($E_h$) of fractional charges from the ground state of the Li atom (N = 3) to the ground state of $Li^-$ (N = 4) and also to the ground state of $Li^+$ (N = 2). LOSC corrections are based on LOSC2 [16].

### 2. *Excited state to ground state electron addition and removal*

TABLE X. The total energies ($E_h$) for the electron removal from the ground state of Li atom (N=3) to the excited states ($(1s)(2s)$) of $Li^+$ (N=2) and also the electron addition to the $Li^-$ (N=4) excited states $(1s)^2(2s)(2p)$. LOSC corrections are based on LOSC2 [16].

| Number of electrons | BLYP total energy | LOSC-BLYP total energy | Exact linearity condition |
|---|---|---|---|
| 2.0 | -5.073435 | -5.073435 | -5.073435 |
| 2.1 | -5.353443 | -5.302755 | -5.314335 |
| 2.2 | -5.628681 | -5.539143 | -5.555236 |
| 2.3 | -5.895516 | -5.778706 | -5.796137 |
| 2.4 | -6.152794 | -6.020133 | -6.037037 |
| 2.5 | -6.400089 | -6.262829 | -6.277938 |
| 2.6 | -6.637174 | -6.506357 | -6.518839 |
| 2.7 | -6.863938 | -6.750357 | -6.759740 |
| 2.8 | -7.080360 | -6.994529 | -7.000640 |
| 2.9 | -7.286493 | -7.238627 | -7.241541 |
| 3.0 | -7.482442 | -7.482442 | -7.482442 |
| 3.1 | -7.485148 | -7.477405 | -7.477942 |
| 3.2 | -7.486374 | -7.472700 | -7.473442 |
| 3.3 | -7.486051 | -7.468124 | -7.468942 |
| 3.4 | -7.484131 | -7.463778 | -7.464443 |
| 3.5 | -7.480577 | -7.459532 | -7.459943 |
| 3.6 | -7.475359 | -7.455316 | -7.455443 |
| 3.7 | -7.468455 | -7.451060 | -7.450943 |
| 3.8 | -7.459845 | -7.446700 | -7.446444 |
| 3.9 | -7.449512 | -7.442175 | -7.441944 |
| 4.0 | -7.437444 | -7.437433 | -7.437444 |

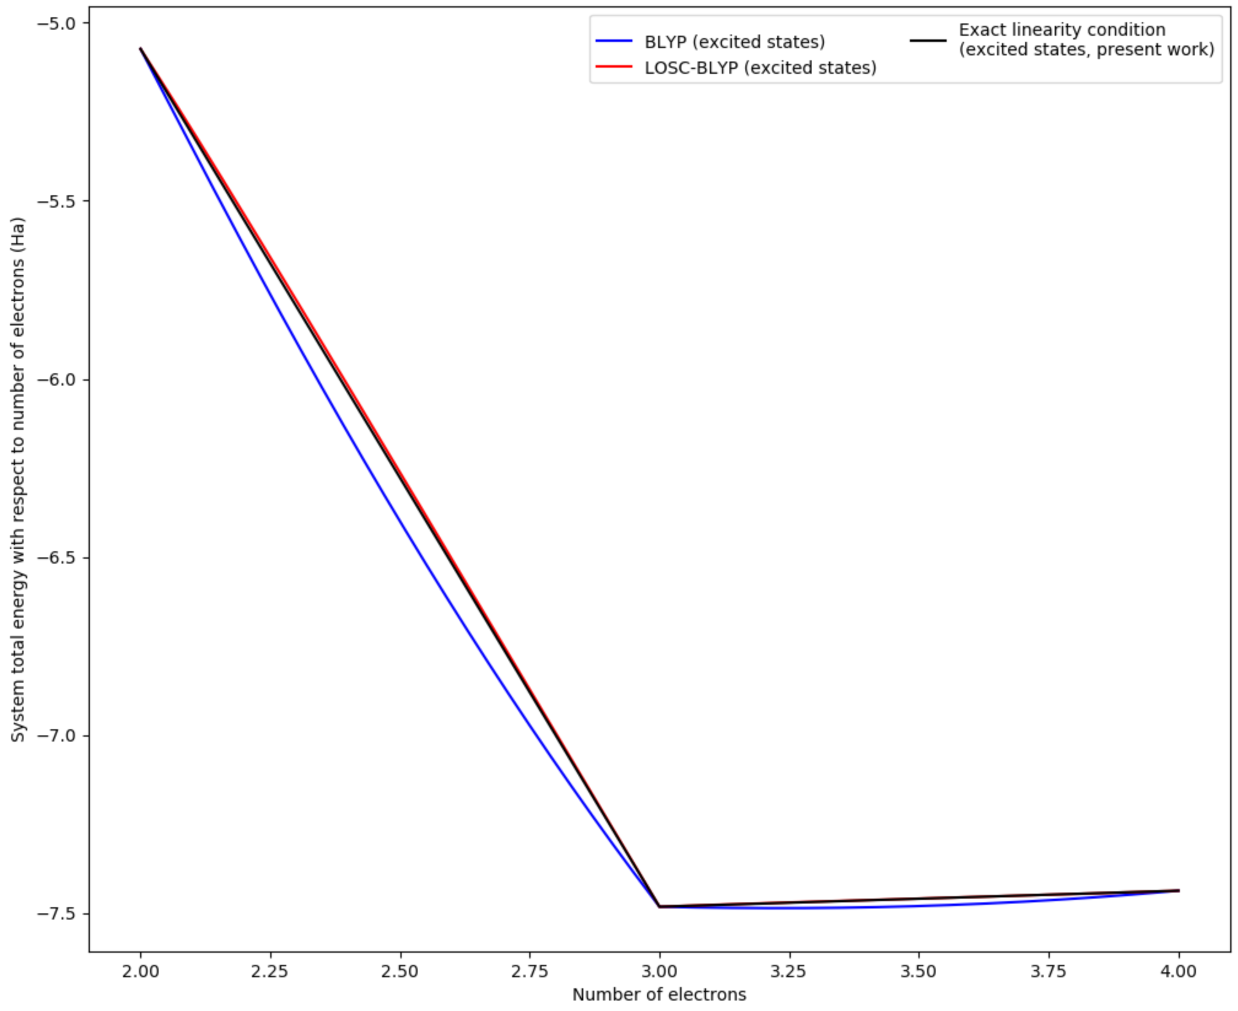


FIG. 6. The total energies ($E_h$) of fractional charges from the ground state of the Li atom (N = 3) to the excited state ($(1s)^2(2s)(2p)$) of $Li^-$ (N = 4) and also to the excited state ($(1s)(2s)$) of $Li^+$ (N = 2). LOSC corrections are based on LOSC2 [16].

## IV. COMPARISON BETWEEN EOM-CCSD AND $\Delta SCF$

### A. OH radical/ion EOM-CCSD and $\Delta SCF$ comparision

The equation of motion coupled-cluster theory (EOM-CCSD) was used to compute the excitation energies for the states of interest. The parent CCSD calculation was performed for the ground state of the OH radical (N=9). The $OH^+$ (N=8) ground state and excited state energies were obtained from the IP-EOM-CCSD subroutine, and the $OH^-$ (N=10) ground state and excited state energies were obtained from the EA-EOM-CCSD subroutine, and the

excited state of OH radical was computed with the Spin-flip excitation (SF-EOM-CCSD) subroutine. All CCSD or EOM-CCSD calculations are implemented in PySCF. All energies are relative to the ground state of OH radical (N = 9), and the ground state energies forOH radical (N = 9) were listed as 0 in the following tables. Def2-TZVPD was used as the basis set for all calculations in this section.

TABLE XI. Ground states $\Delta SCF$ and EOM-CCSD energies relative to the OH radical (N=9) ground state, units are in eV

| | $\Delta LDA$ | $\Delta BLYP$ | $\Delta B3LYP$ | EOM-CCSD |
|---|---|---|---|---|
| $OH^+$ (N=8) ground state | 13.48 | 13.28 | 13.30 | 12.85 |
| OH radical (N=9) ground state | 0 | 0 | 0 | 0 |
| $OH^-$ (N=10) ground state | -2.37 | -1.96 | -1.84 | -1.52 |

TABLE XII. Excited states $\Delta SCF$ and EOM-CCSD energies relative to the OH radical (N=9) ground state, units are in eV

| | $\Delta LDA$ | $\Delta BLYP$ | $\Delta B3LYP$ | EOM-CCSD |
|---|---|---|---|---|
| $OH^+$ (N=8) excited state | 17.05 | 16.88 | 16.92 | 16.66 |
| OH radical (N=9) excited state | 11.05 | 10.94 | N/A | 10.41 |
| $OH^-$ (N=10) excited state | 1.39 | 1.55 | 1.46 | 1.69 |

## B. Li atom/ion EOM-CCSD and $\Delta SCF$ comparision

Similar to the calculation for OH related systems, the excitation energies were obtained from EOM-CCSD theory. The parent CCSD calculation was perfromed for the Li atom (N=3) ground state, and the energies for $Li^+$ cation (N=2) were obtained from IP-EOM-CCSD subroutine, and the energies for $Li^+$ anion (N=4) were obtained from EA-EOM-CCSD subroutine. All energies were relative to the ground state of Li atom (N=3), and the ground state energies for Li atom (N=3) were listed as 0 in the following tables. Def2-TZVPD was used as the basis set for all calculations in this section.

TABLE XIII. Ground states $\Delta SCF$ and EOM-CCSD energies relative to the Li atom (N=3) ground state, units are in eV

| | $\Delta LDA$ | $\Delta BLYP$ | EOM-CCSD |
|---|---|---|---|
| $Li^+$ (N=2) ground state | 5.47 | 5.53 | 5.37 |
| Li atom (N=3) ground state | 0 | 0 | 0 |
| $Li^-$ (N=4) ground state | -0.39 | -0.22 | -0.45 |

TABLE XIV. Excited states $\Delta SCF$ and EOM-CCSD energies relative to the Li atom (N=3) ground state, units are in eV

| | $\Delta LDA$ | $\Delta BLYP$ | EOM-CCSD |
|---|---|---|---|
| $Li^+$ (N=2) excited state | 64.59 | 65.55 | 64.73 |
| $Li^-$ (N=4) excited state | 0.29 | 1.22 | 0.46 |


[1] I. Mayer, *Simple Theorems, Proofs, and Derivations in Quantum Chemistry*, edited by P. G. Mezey, Mathematical and Computational Chemistry (Springer US, Boston, MA, 2003).

[2] M. Nakata and J. S. M. Anderson, On the size-consistency of the reduced-density-matrix method and the unitary invariant diagonal N-representability conditions, AIP Advances **2**, 032125 (2012).

[3] R. G. Parr and W. Yang, Density functional approach to the frontier-electron theory of chemical reactivity, Journal of the American Chemical Society **106**, 4049 (1984), 02059.

[4] R. G. Parr and R. G. Pearson, Absolute hardness: companion parameter to absolute electronegativity, Journal of the American Chemical Society **105**, 7512 (1983), 04491.

[5] R. G. Parr, R. A. Donnelly, M. Levy, and W. E. Palke, Electronegativity: the density functional viewpoint, The Journal of Chemical Physics **68**, 3801 (1978).

[6] P. Geerlings, F. De Proft, and W. Langenaeker, Conceptual Density Functional Theory, Chemical Reviews **103**, 1793 (2003), publisher: American Chemical Society.

[7] S. H. Vosko, L. Wilk, M. Nusair, S. H. Vosko, L. Wilk, and M. Nusair, Accurate spin-dependent electron liquid correlation energies for local spin density calculations: a critical analysis, CaJPh **59**, 1200 (1980).

[8] A. D. Becke, Density-functional exchange-energy approximation with correct asymptotic behavior, Phys. Rev. A **38**, 3098 (1988).

[9] C. Lee, W. Yang, and R. G. Parr, Development of the colle-salvetti correlation-energy formula into a functional of the electron density, Phys. Rev. B **37**, 785 (1988).

[10] P. J. Stephens, F. J. Devlin, C. F. Chabalowski, and M. J. Frisch, Ab initio calculation of vibrational absorption and circular dichroism spectra using density functional force fields, J. Phys. Chem. **98**, 11623 (1994).

[11] An in-house program for qm/mm simulations. https://qm4d.org/.

[12] Q. Sun, T. C. Berkelbach, N. S. Blunt, G. H. Booth, S. Guo, Z. Li, J. Liu, J. D. McClain, E. R. Sayfutyarova, S. Sharma, S. Wouters, and G. K. L. Chan, Pyscf: the python-based simulations of chemistry framework, Wiley Interdisciplinary Reviews: Computational Molecular Science **8**, e1340 (2018).

[13] Q. Sun, X. Zhang, S. Banerjee, P. Bao, M. Barbry, N. S. Blunt, N. A. Bogdanov, G. H. Booth, J. Chen, Z. H. Cui, J. J. Eriksen, Y. Gao, S. Guo, J. Hermann, M. R. Hermes, K. Koh, P. Koval, S. Lehtola, Z. Li, J. Liu, N. Mardirossian, J. D. McClain, M. Motta, B. Mussard, H. Q. Pham, A. Pulkin, W. Purwanto, P. J. Robinson, E. Ronca, E. R. Sayfutyarova, M. Scheurer, H. F. Schurkus, J. E. Smith, C. Sun, S. N. Sun, S. Upadhyay, L. K. Wagner, X. Wang, A. White, J. D. Whitfield, M. J. Williamson, S. Wouters, J. Yang, J. M. Yu, T. Zhu, T. C. Berkelbach, S. Sharma, A. Y. Sokolov, and G. K. L. Chan, Recent developments in the p y scf program package, J. Chem. Phys. **153**, 24109 (2020).

[14] A. T. B. Gilbert, N. A. Besley, and P. M. W. Gill, Self-consistent field calculations of excited states using the maximum overlap method (MOM), J. Phys. Chem. A **112**, 13164 (2008).

[15] P. Mori-Sánchez, A. J. Cohen, and W. Yang, Many-electron self-interaction error in approximate density functionals, The Journal of Chemical Physics **125**, 201102 (2006).

[16] N. Q. Su, A. Mahler, and W. Yang, Preserving symmetry and degeneracy in the localized orbital scaling correction approach, J. Phys. Chem. Lett. **11**, 1528 (2020).

[17] Y. Mei, Z. Chen, and W. Yang, Exact second-order corrections and accurate quasiparticle energy calculations in density functional theory, J. Phys. Chem. Lett. **12**, 7236 (2021).

[18] J. Yu, Y. Mei, Z. Chen, and W. Yang, Accurate Prediction of Core Level Binding Energies from Ground-State Density Functional Calculations: The Importance of Localization and Screening (2024), arXiv:2406.06345 [physics].

[19] J. Z. Williams and W. Yang, Correcting Delocalization Error in Materials with Localized Orbitals and Linear-Response Screening (2024), arXiv:2406.07351 [cond-mat, physics:physics].

[20] C. Li, J. Lu, and W. Yang, On extending Kohn-Sham density functionals to systems with fractional number of electrons, J. Chem. Phys. **146**, 10.1063/1.4982951 (2017).

[21] D. Rappoport and F. Furche, Property-optimized gaussian basis sets for molecular response calculations, J. Chem. Phys. **133**, 134105 (2010).

[22] F. Weigend and R. Ahlrichs, Balanced basis sets of split valence, triple zeta valence and quadruple zeta valence quality for h to rn: Design and assessment of accuracy, Phys. Chem. Chem. Phys. **7**, 3297 (2005).
